# Supplementary material for: Canonical thresholding for non-sparse high-dimensional linear regression
Source: arXiv:2007.12313 source file (2021-09-30)
Supplement: Supplementary file 1 [file bibliography_supp.tex]

%
%\bibitem[Bair et al.(2006)]{SPCR}
%\textsc{Bair, E.}, \textsc{Hastie, T.}, \textsc{Paul, D.} and \textsc{Tibshirani, R.} (2006).
%Prediction by supervised principal components.
%\textit{J. Amer. Statist. Assoc.},  \textbf{101}, 473, 119--137.
%
\bibitem[Bartlett et al.(2020)]{Bartlett}
\textsc{Bartlett, P.}, \textsc{Long, P.}, \textsc{Lugosi, G.} and \textsc{Tsigler, A.} (2020).
Benign overfitting in linear regression.
\textit{Proc. Natl. Acad. Sci. USA}.
%
%\bibitem[Belkin(2018)]{BelkinPMLR}
%\textsc{Belkin, M.} (2018).
%Approximation beats concentration? An approximation view on inference with smooth radial kernels.
%\textit{Proc. Mach. Learn. Res.}, \textbf{75}, 1--18.
%
%\bibitem[Belkin, Hsu and Xu(2019)]{Belkin}
%\textsc{Belkin, M.}, \textsc{Hsu, D.} and \textsc{Xu, J.} (2019).
%Two models of double descent for weak features.
%\textit{ArXiv:1903.07571}.
%
%\bibitem[Bellec, Lecué and Tsybakov(2018)]{SLOPE2}
%\textsc{Bellec, P.}, \textsc{Lecué, G.} and \textsc{Tsybakov, A.} (2018).
%SLOPE meets Lasso: improved oracle bounds and optimality.
%\textit{Ann. Statist.},
%\textbf{46}, 6B, 3603--3642.
%
%\bibitem[Bickel, Ritov and Tsybakov(2009)]{Dantzig2}
%\textsc{Bickel, P.}, \textsc{Ritov, Y.} and \textsc{Tsybakov, A.} (2009).
%Simultaneous analysis of Lasso and Dantzig selector.
%\textit{Ann. Statist.},
%\textbf{37}, 4, 1705--1732.
%
%\bibitem[Bietti and Mairal(2019)]{NTK}
%\textsc{Bietti, A.} and \textsc{Mairal, J.} (2019).
%On the inductive bias of Neural Tangent Kernels.
%\textit{Advances in Neural Information Processing Systems}, 12893--12904.
%
%\bibitem[Bogdan et al.(2015)]{SLOPE}
%\textsc{Bogdan, M.}, \textsc{van den Berg, E.}, \textsc{Sabatti, C.}, \textsc{Su, W.} and \textsc{Candes, E.} (2015).
%SLOPE -- adaptive variable selection via convex optimization.
%\textit{Ann. Appl. Stat.},
%\textbf{9}, 3, 1103--1140.
%
\bibitem[Cardot, Mas and Sarda(2007)]{Cardot}
\textsc{Cardot, H.}, \textsc{Mas, A.} and \textsc{Sarda, P.} (2007).
CLT in functional linear regression models.
\textit{Probab. Theory Related Fields},  \textbf{138}, 325--361.
\bibitem[Dudoit and van der Laan(2005)]{CV}
\textsc{Dudoit, S.} and \textsc{van der Laan, M. J.} (2005).
Asymptotics of cross-validated risk estimation in estimator selection and performance assessment.
\textit{Statist. Methodol.},
\textbf{2}, 2, 131--154.

\bibitem[Jirak(2016)]{Jirak}
\textsc{Jirak, M.} (2016).
Optimal eigen expansions and uniform bounds.
\textit{Probab. Theory Related Fields},
\textbf{166}, 753--799.
\bibitem[Jirak and Wahl(2018)]{Wahl}
\textsc{Jirak, M.} and \textsc{Wahl, M.} (2018).
Relative perturbation bounds with applications to empirical covariance operators.
\textit{ArXiv:1802.02869}.

\bibitem[Johnstone(2019)]{Draft}
\textsc{Johnstone, I. M.} (2019).
Gaussian estimation: Sequence and wavelet models. \textit{Draft}.
\url{statweb.stanford.edu/~imj/GE_09_16_19.pdf}. 
%
%
%\bibitem[Jolliffe(1982)]{Jolliffe}
%\textsc{Jolliffe, I.} (1982).
%A note on the use of principal components in regression.
%\textit{J. R. Stat. Soc. Ser. C. Appl. Stat.},
%\textbf{31}, 3, 300--303.
%
\bibitem[Koltchinskii and Lounici(2017)]{Koltchinskii_CIAMBFSCO}
\textsc{Koltchinskii, V.} and \textsc{Lounici, K.} (2017).
Concentration inequalities and moment bounds for sample covariance operators.
\textit{Bernoulli},
\textbf{23}, 1, 110--133.
\bibitem[Kuchibhotla and Chakrabortty(2018)]{Weibull}
\textsc{Kuchibhotla, A. K.} and \textsc{Chakrabortty, A.} (2018).
Moving beyond sub-Gaussianity in high-dimensional statistics: applications in covariance estimation and linear regression.
\textit{ArXiv:1804.02605}.
%
%\bibitem[Liang and Rakhlin(2020)]{Rakhlin}
%\textsc{Liang, T.} and \textsc{Rakhlin, A.} (2020).
%Just interpolate: kernel ''ridgeless'' regression can generalize.
%\textit{Ann. Statist.}, \textbf{48}, 3, 1329--1347.
%
%\bibitem[Ma and Belkin(2017)]{EigenPro}
%\textsc{Ma, S.} and \textsc{Belkin, M.} (2017).
%Diving into the shallows: a computational perspective on large-scale shallow learning.
%\textit{Advances in Neural Information Processing Systems}, 3781--3790.
%
%\bibitem[Paul et al.(2008)]{Precond}
%\textsc{Paul, D.}, \textsc{Bair, E.}, \textsc{Hastie, T.} and \textsc{Tibshirani, R.} (2008).
%``Preconditioning'' for feature selection and regression in high-dimensional problems.
%\textit{Ann. Statist.}, \textbf{36}, 4, 1595--1618.
%
%\bibitem[Pearson(1901)]{Pearson}
%\textsc{Pearson, K.} (1901).
%On lines and planes of closest fit to systems of points in space.
%\textit{The London, Edinburgh and Dublin Philosophical Magazine and Journal of Science.},
%\textbf{2}, 559--572.

\bibitem[Rigollet(2019)]{Rigollet}
\textsc{Rigollet, P.} (2019).
\textit{Lecture notes on High-dimensional statistics}.
%
%\bibitem[Tibshirani(1996)]{LASSO}
%\textsc{Tibshirani, R.} (1996).
%Regression shrinkage and selection via the Lasso.
%\textit{J. R. Stat. Soc. Ser. B. Stat. Methodol.},
%\textbf{58}, 1, 267--288.

\bibitem[Tsybakov(2009)]{Tsybakov}
\textsc{Tsybakov, A. B.} (2009). 
Introduction to nonparametric estimation.
\textit{Springer Series in Statistics}, Springer, New York.
%
%\bibitem[van de Geer and Bühlmann(2009)]{vandeGeer}
%\textsc{van de Geer, S.} and \textsc{Bühlmann, P.} (2009).
%On the conditions used to prove oracle results for the Lasso.
%\textit{Electron. J. Stat.},
%\textbf{3}, 1360--1392.
%
\bibitem[Vershynin(2018)]{Vershynin}
\textsc{Vershynin, R.} (2018).
High-dimensional probability.
An introduction with applications in data science.
\textit{Cambridge Series in Statistical and Probabilistic Mathematics}.
%
%\bibitem[Zumbach(2009)]{FinData1}
%\textsc{Zumbach, G.} (2009).
%The empirical properties of large covariance matrices.
%\textit{RiskMetrics Journal}, \textbf{9}, 1.
